# Supplementary material for: RegionCL: Can Simple Region Swapping Contribute to Contrastive Learning?
Source: arXiv:2111.12309 source file (2022-11-10)
Supplement: Supplementary file 1 [file Supp_Tab_ViT.tex]

% Table generated by Excel2LaTeX from sheet 'Longer Epochs'
\begin{table}[htbp]
  \centering
  \footnotesize
  \caption{Results of MoCo v3~\cite{} and \modelName-M with ViT-S~\cite{}.}
    \begin{tabular}{l|c|cc}
    \hline
          & \multirow{2}[2]{*}{Epochs} & \multicolumn{2}{c}{ImageNet} \\
          &       & Top-1 & Top-5 \\
    \hline
    MoCo v3 & 300   & 72.5  & - \\
    \modelName-M & 300   &       &  \\
    \hline
    \end{tabular}%
  \label{tab:supp_vit}%
\end{table}%
